# Supplementary material for: Unbiased Learning of Deep Generative Models with Structured Discrete Representations
Source: arXiv:2306.08230 source file (2023-11-14)
Supplement: Supplementary file 1 [file neurips_appendix.tex]

\documentclass{article}
\usepackage{bm}

% if you need to pass options to natbib, use, e.g.:
%     \PassOptionsToPackage{numbers, compress}{natbib}
% before loading neurips_2020

% ready for submission
% \usepackage{neurips_2020}

% to compile a preprint version, e.g., for submission to arXiv, add add the
% [preprint] option:
%     \usepackage[preprint]{neurips_2020}

% to compile a camera-ready version, add the [final] option, e.g.:
%     \usepackage[final]{neurips_2023}
\PassOptionsToPackage{square,numbers}{natbib}

% to avoid loading the natbib package, add option nonatbib:
     \usepackage{neurips_2023}

\usepackage[utf8]{inputenc} % allow utf-8 input
\usepackage[T1]{fontenc}    % use 8-bit T1 fonts
\usepackage{hyperref}       % hyperlinks
\hypersetup{
    colorlinks,
    citecolor=blue,
    filecolor=blue,
    linkcolor=blue,
    urlcolor=black,
}
\usepackage{url}            % simple URL typesetting
\usepackage{booktabs}       % professional-quality tables
\usepackage{amsfonts}       % blackboard math symbols
\usepackage{nicefrac}       % compact symbols for 1/2, etc.
\usepackage{microtype}      % microtypography
\usepackage[dvipsnames]{xcolor}         % colors
\usepackage{overpic}
\usepackage{subfigure}
\usepackage{array}
\definecolor{ao}{rgb}{0.0, 0.5, 0.0}

\PassOptionsToPackage{noend}{algorithmic}
\RequirePackage{algorithm}
\RequirePackage{algorithmic}

\usepackage{amsthm}
\theoremstyle{plain}

\theoremstyle{definition}

\theoremstyle{remark}

\bibliographystyle{icml2021}

\usepackage{mathtools}
   % rbp

\DeclarePairedDelimiterX{\infdivx}[2]{(}{)}{%
  #1\;\delimsize\|\;#2%
}

\usepackage{bbm}
\usepackage{bm}

\title{Unbiased Learning of Deep Generative Models\\with Structured Discrete Representations: Supplementary Materials}

% The \author macro works with any number of authors. There are two commands
% used to separate the names and addresses of multiple authors: \And and \AND.
%
% Using \And between authors leaves it to LaTeX to determine where to break the
% lines. Using \AND forces a line break at that point. So, if LaTeX puts 3 of 4
% authors names on the first line, and the last on the second line, try using
% \AND instead of \And before the third author name.

\author{%
  David S.~Hippocampus\thanks{Use footnote for providing further information
    about author (webpage, alternative address)---\emph{not} for acknowledging
    funding agencies.} \\
  Department of Computer Science\\
  Cranberry-Lemon University\\
  Pittsburgh, PA 15213 \\
  \texttt{hippo@cs.cranberry-lemon.edu} \\
  % examples of more authors
  % \And
  % Coauthor \\
  % Affiliation \\
  % Address \\
  % \texttt{email} \\
  % \AND
  % Coauthor \\
  % Affiliation \\
  % Address \\
  % \texttt{email} \\
  % \And
  % Coauthor \\
  % Affiliation \\
  % Address \\
  % \texttt{email} \\
  % \And
  % Coauthor \\
  % Affiliation \\
  % Address \\
  % \texttt{email} \\
}

\begin{document}

% Reset vertical space for displayed equations 
% (must be after \begin{document})
\setlength{\abovedisplayskip}{2pt plus 3pt}
\setlength{\belowdisplayskip}{2pt plus 3pt}

\maketitle

% \begin{abstract}
% By composing graphical models with deep learning architectures, we learn generative models with the strengths of both frameworks. 
% %A prominent synthesizer of these two techniques is 
% The structured variational autoencoder (SVAE) inherits structure and interpretability from graphical models, and flexible likelihoods for high-dimensional data from deep learning, but poses substantial optimization challenges.  We propose novel algorithms for learning SVAEs, and are the first to demonstrate the SVAE's ability to handle multimodal uncertainty when data is missing by incorporating discrete latent variables.  
% %capabilities to handle missing data and multi-modality better than state-of-the-art deep learning models. 
% Our memory-efficient implicit differentiation scheme makes the SVAE tractable to learn via gradient descent, while demonstrating robustness to incomplete optimization. To more rapidly learn accurate graphical model parameters, we derive a method for computing natural gradients without manual derivations, which avoids biases found in prior work.  These optimization innovations enable the first comparisons of the SVAE to state-of-the-art time series models, where the SVAE performs competitively while learning interpretable and structured discrete data representations.
% \end{abstract}
\appendix

\section{Experimental Protocol}
\newcommand{\panelWidth}{4.6cm} %% width of each image
\setlength{\tabcolsep}{0.01cm}  %% space between columns
\begin{figure*}[!t]
\centering
\begin{tabular}{p{\panelWidth} p{\panelWidth} p{\panelWidth} }
\begin{overpic}[width=\panelWidth]{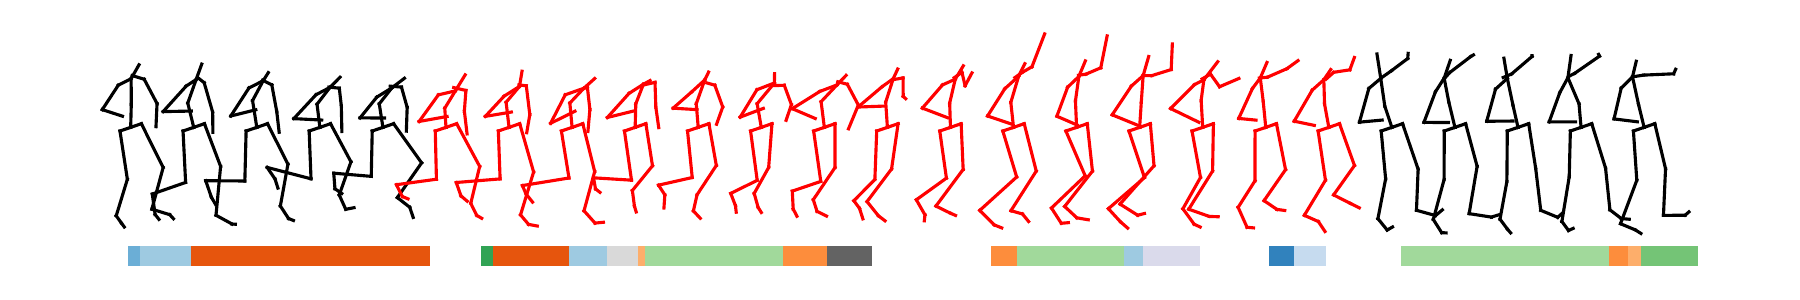}
\end{overpic} &
\begin{overpic}[width=\panelWidth]{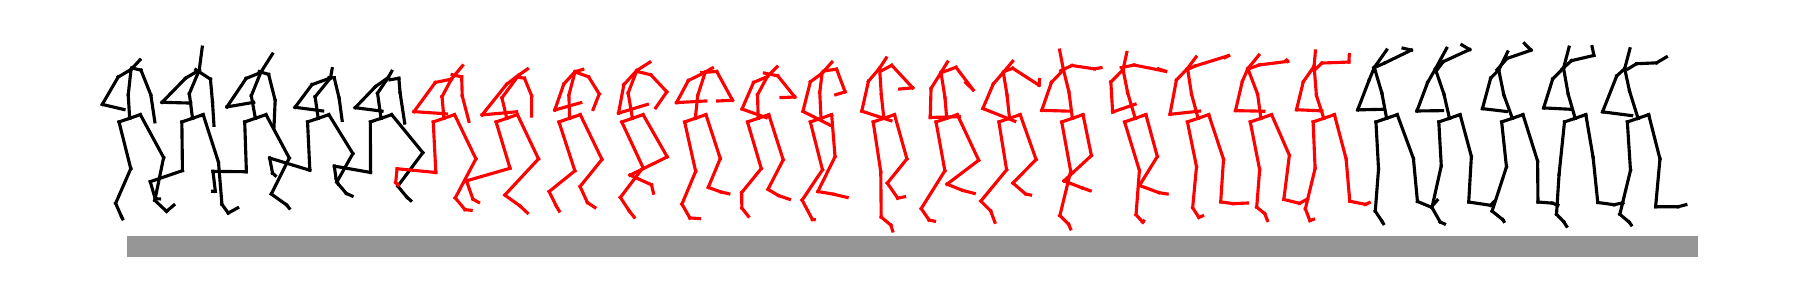}
\end{overpic} &
\begin{overpic}[width=\panelWidth]{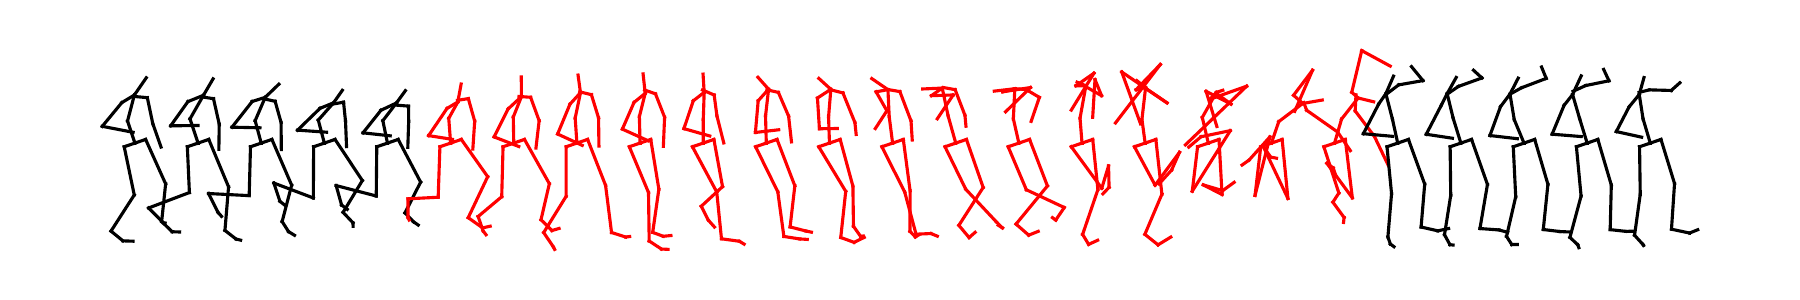}
\end{overpic} \\
\begin{overpic}[width=\panelWidth]{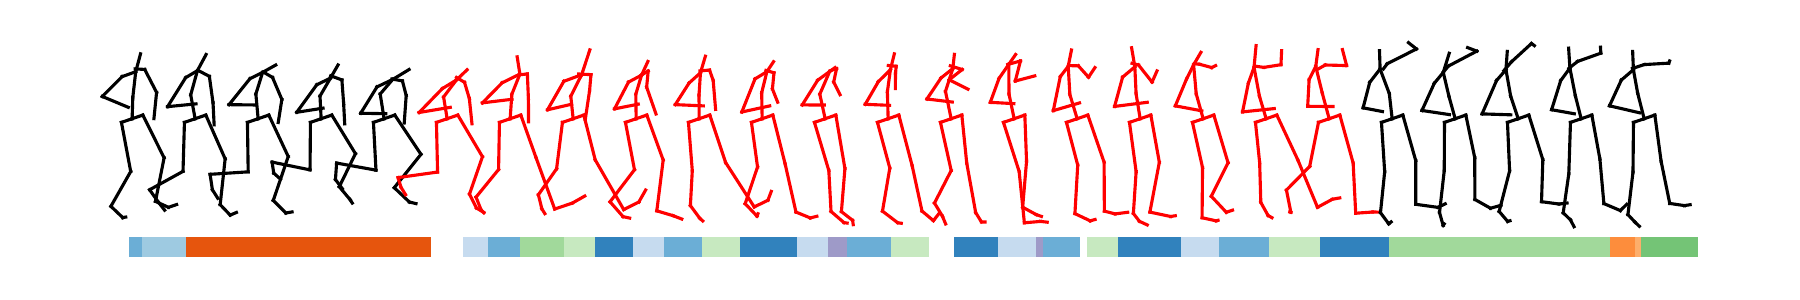}
\end{overpic} &
\begin{overpic}[width=\panelWidth]{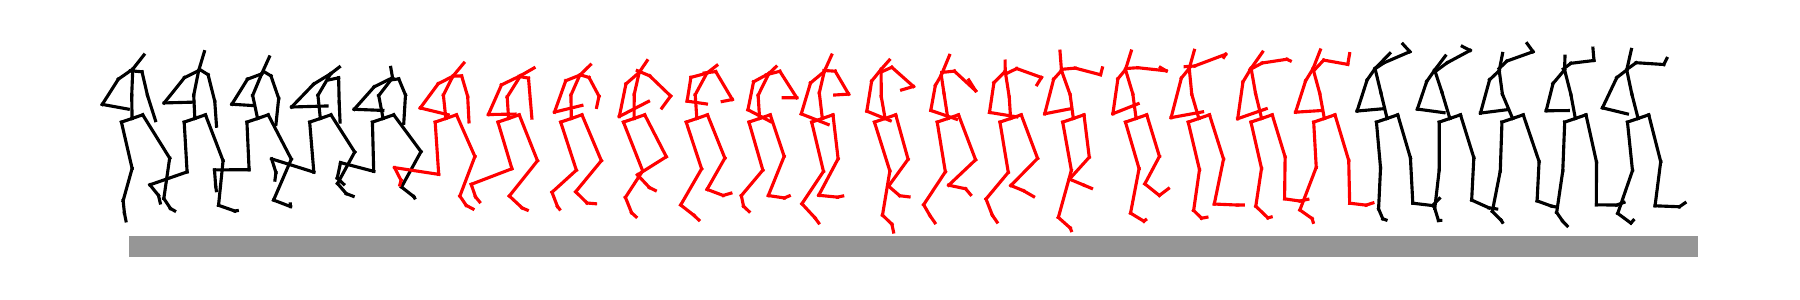}
\end{overpic} &
\begin{overpic}[width=\panelWidth]{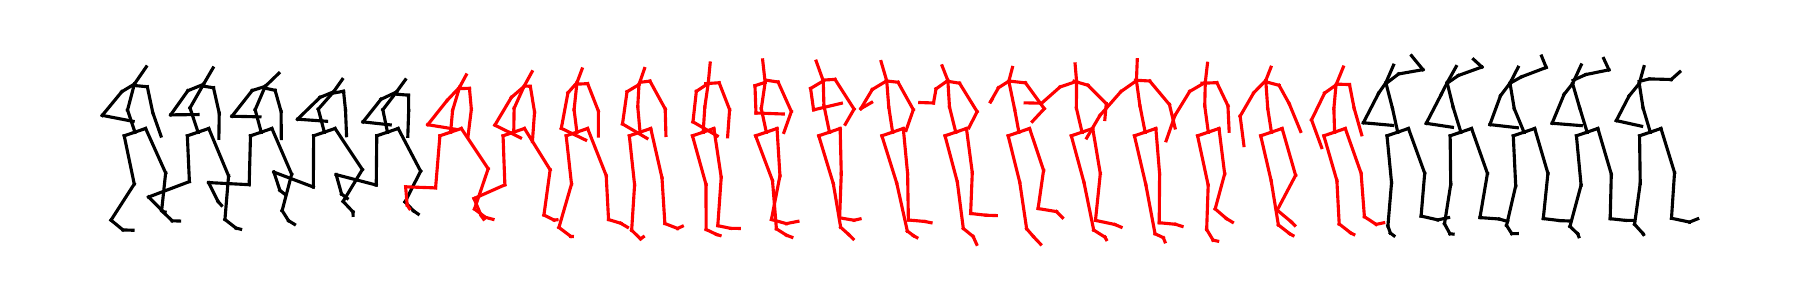}
\end{overpic} \\
\begin{overpic}[width=\panelWidth]{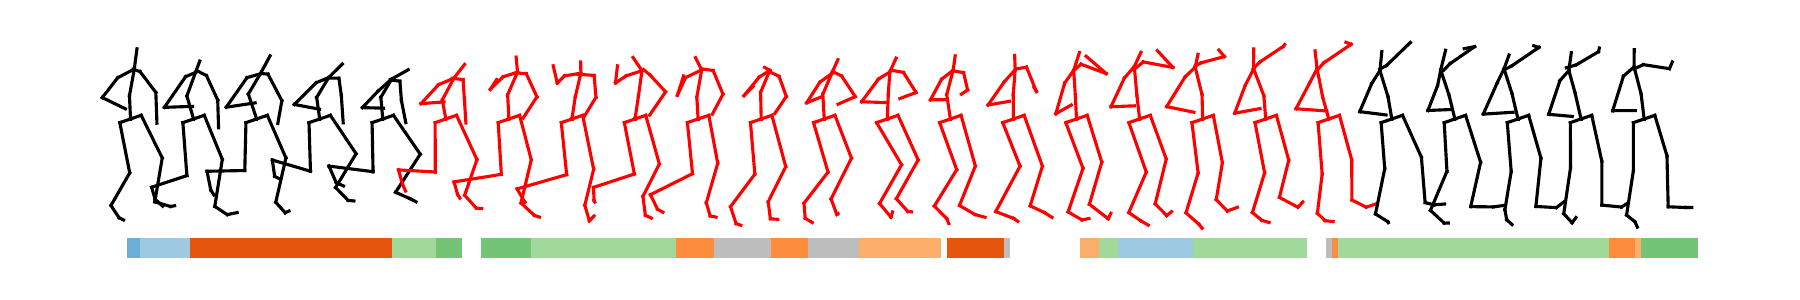}
\end{overpic} &
\begin{overpic}[width=\panelWidth]{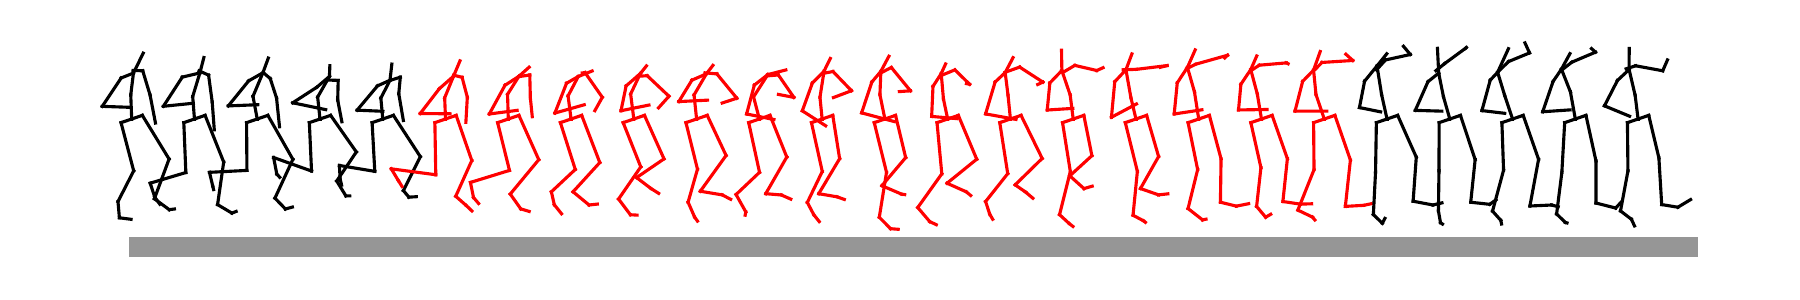}
\end{overpic}
&
\begin{overpic}[width=\panelWidth]{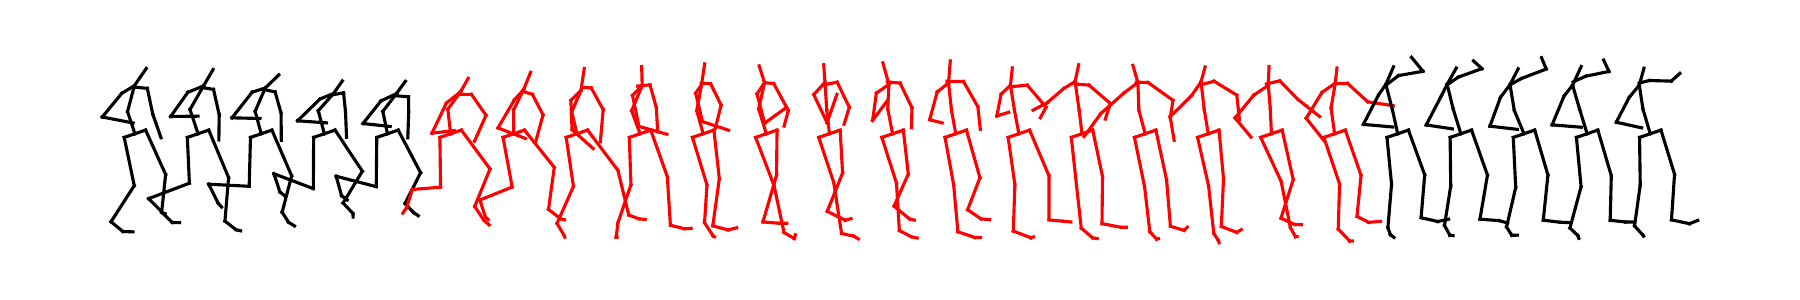}
\end{overpic} \\
\begin{overpic}[width=\panelWidth]{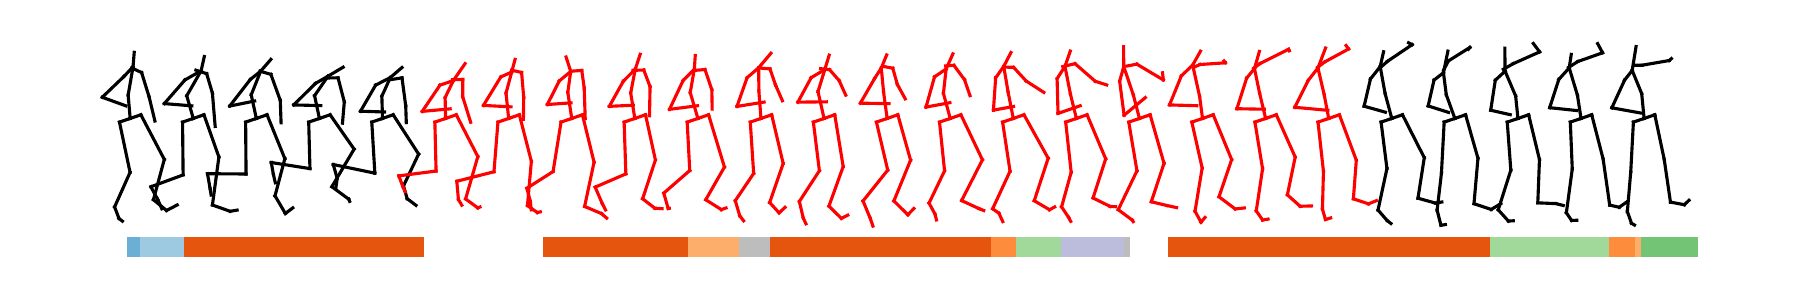}
\end{overpic} &
\begin{overpic}[width=\panelWidth]{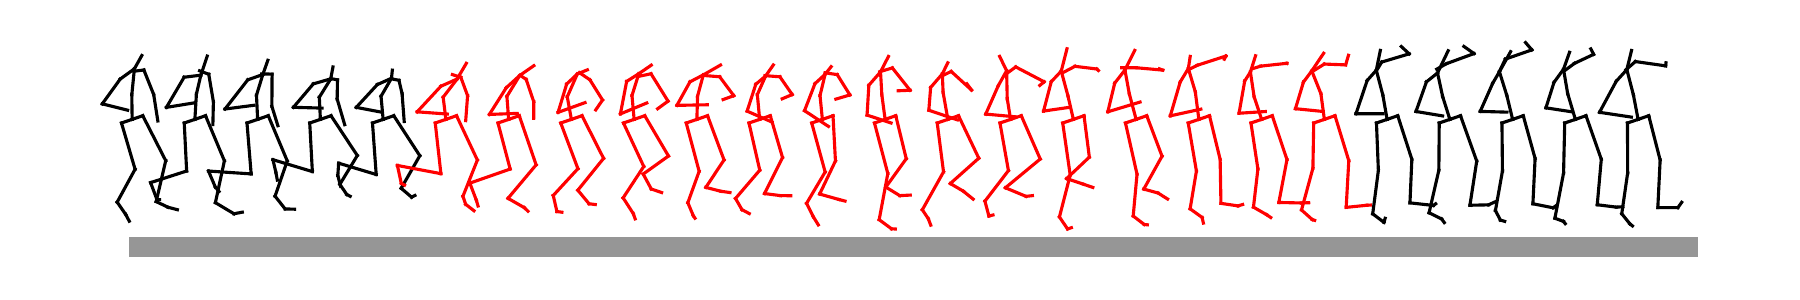}
\end{overpic} &
\begin{overpic}[width=\panelWidth]{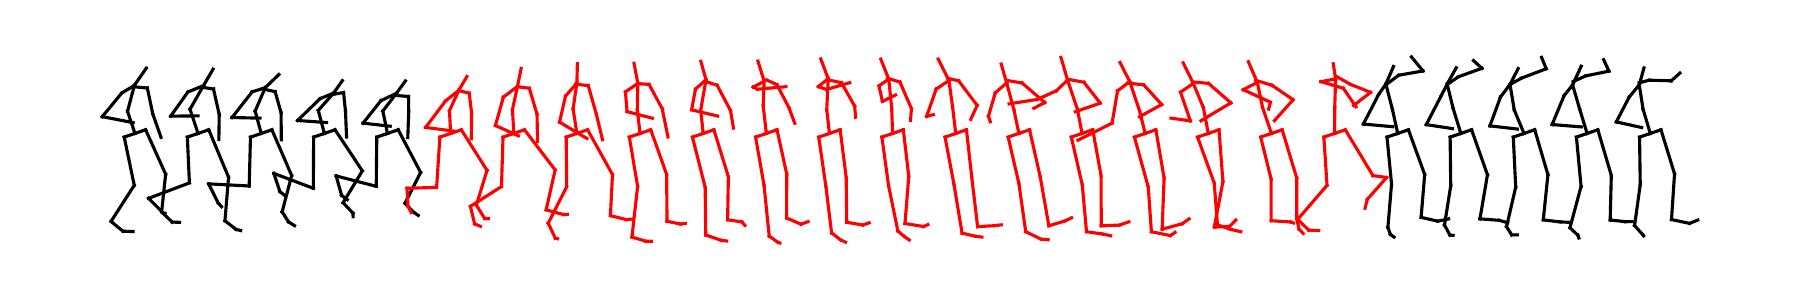}
\end{overpic}
\end{tabular}
(SVAE-SLDS) \hspace{20mm} (SVAE-SLDS-bias) \hspace{24mm} (SRNN)\\
\begin{tabular}{p{\panelWidth} p{\panelWidth} p{\panelWidth} }
\begin{overpic}[width=\panelWidth]{figs/interpolations/interpolation_transformer3_0.pdf}
\end{overpic} &
\begin{overpic}[width=\panelWidth]{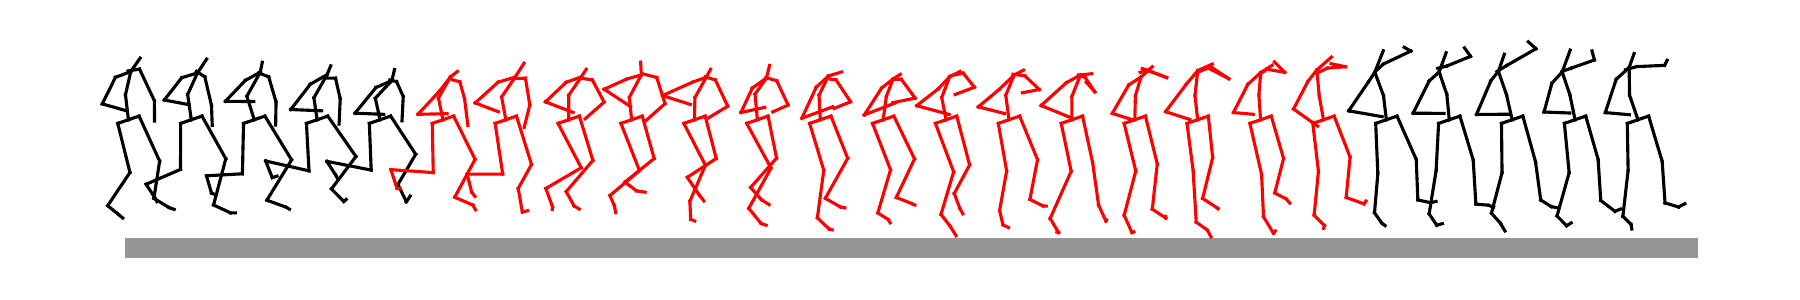}
\end{overpic} &
\begin{overpic}[width=\panelWidth]{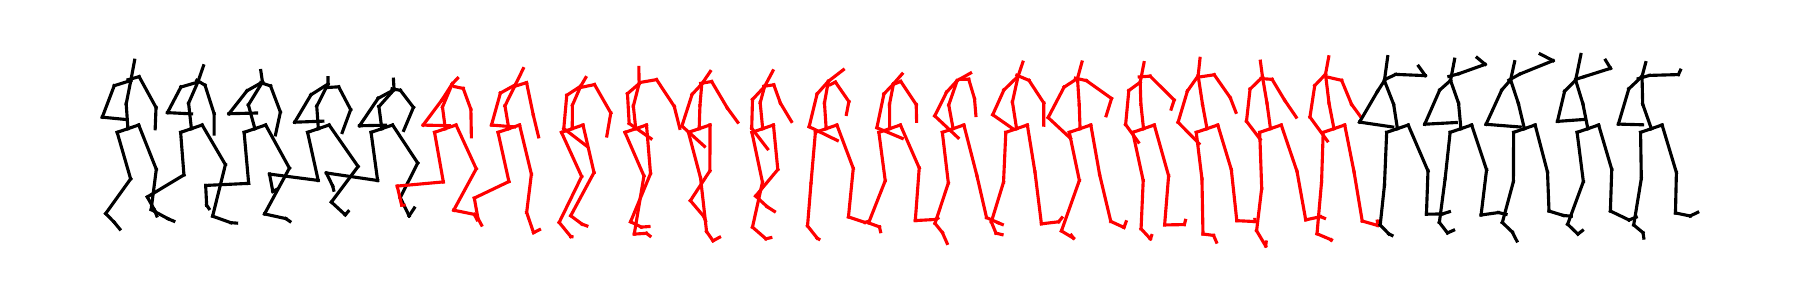}
\end{overpic} \\
\begin{overpic}[width=\panelWidth]{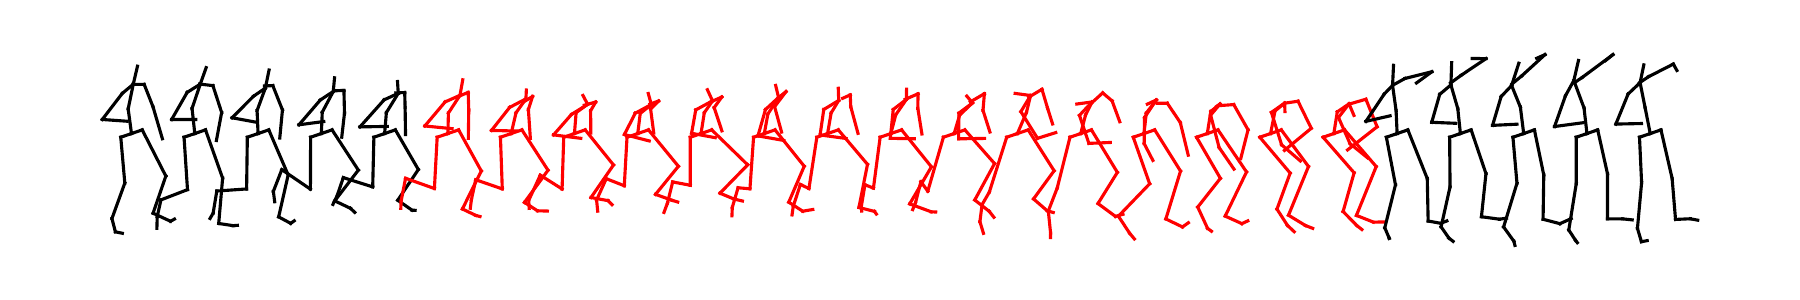}
\end{overpic} &
\begin{overpic}[width=\panelWidth]{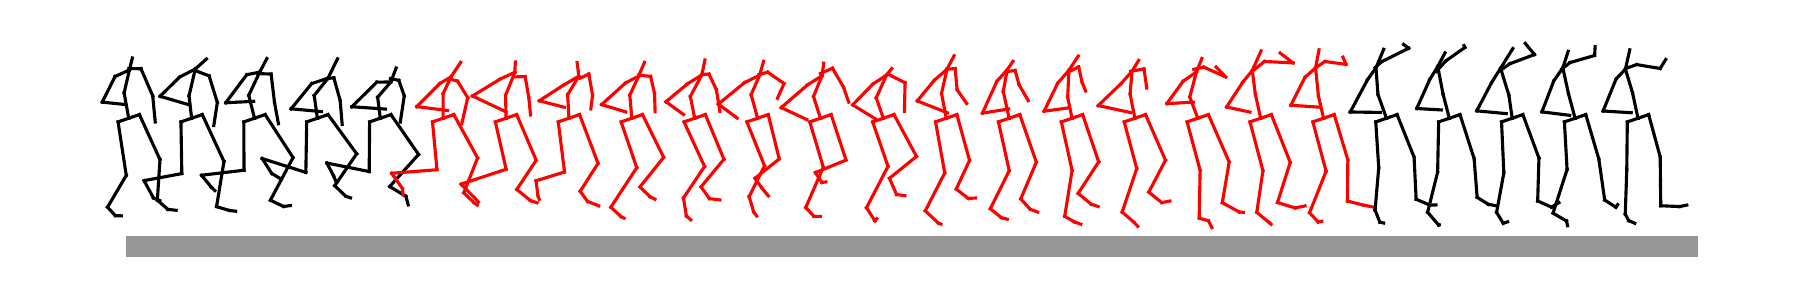}
\end{overpic} &
\begin{overpic}[width=\panelWidth]{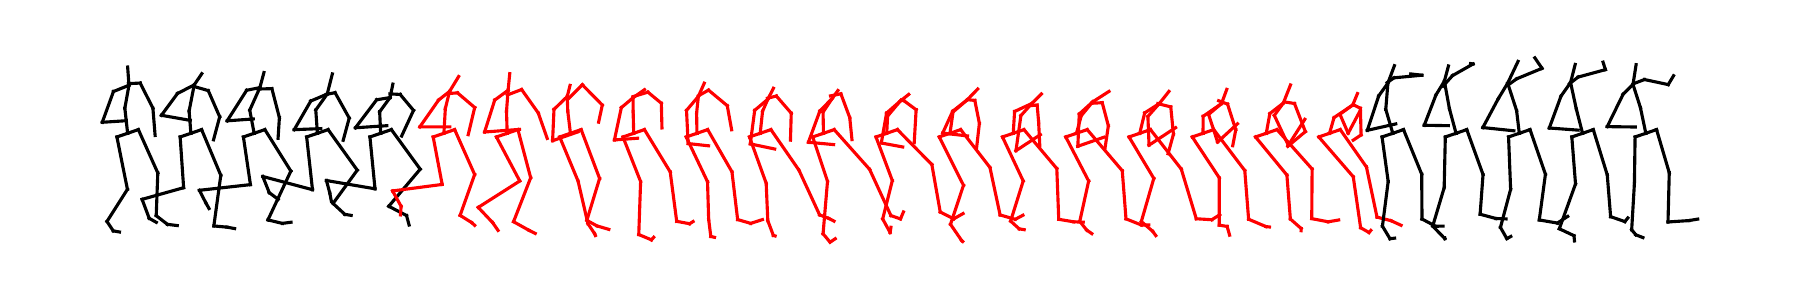}
\end{overpic} \\
\begin{overpic}[width=\panelWidth]{figs/interpolations/interpolation_transformer3_2.pdf}
\end{overpic} &
\begin{overpic}[width=\panelWidth]{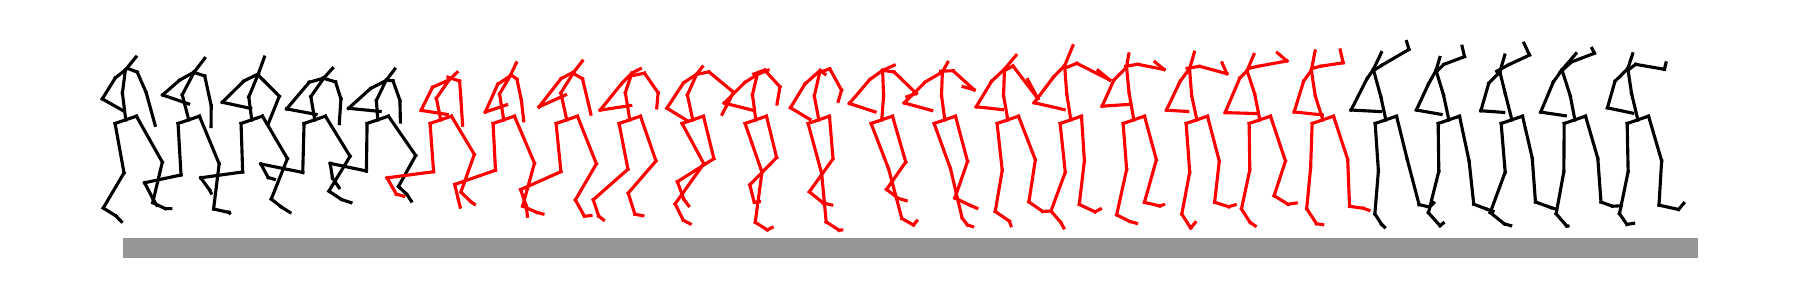}
\end{overpic}
&
\begin{overpic}[width=\panelWidth]{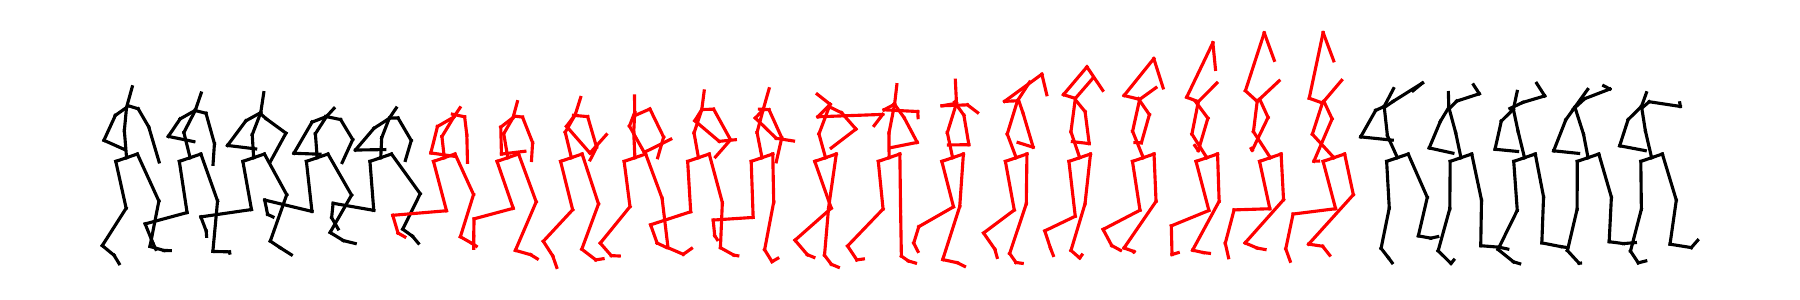}
\end{overpic} \\
\begin{overpic}[width=\panelWidth]{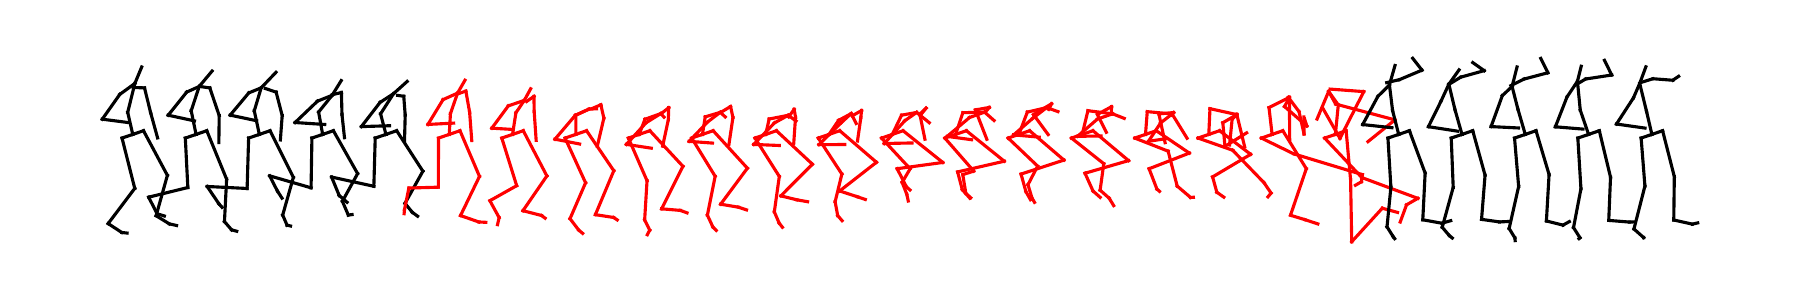}
\end{overpic} &
\begin{overpic}[width=\panelWidth]{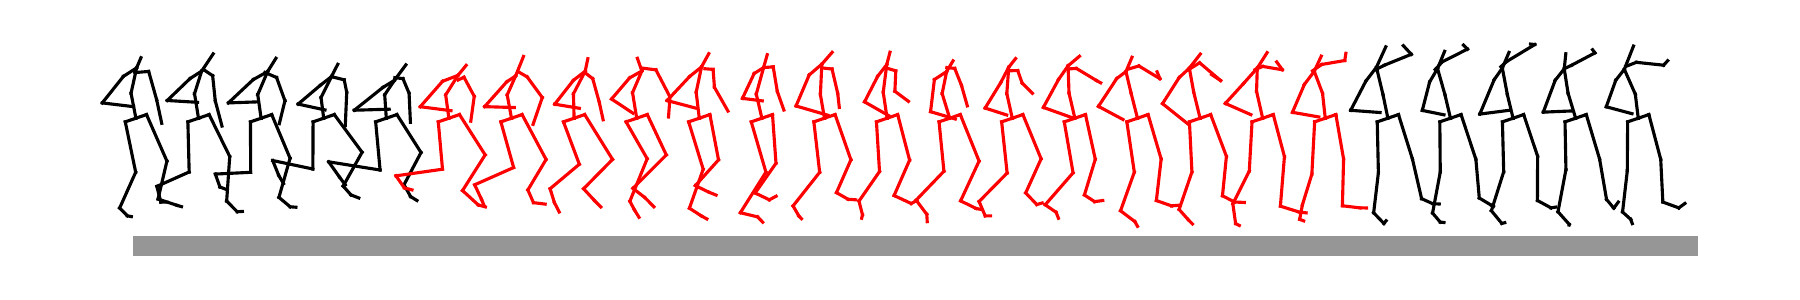}
\end{overpic} &
\begin{overpic}[width=\panelWidth]{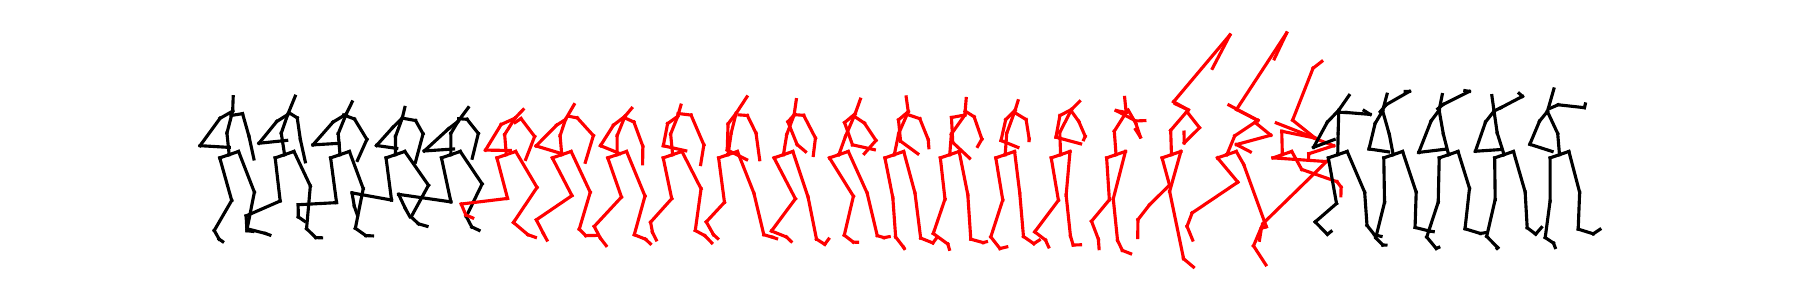}
\end{overpic}
\end{tabular}
(Transformer) \hspace{20mm} (SIN-SLDS) \hspace{24mm} (DKS)\\
\begin{tabular}{p{\panelWidth} p{\panelWidth} p{\panelWidth} }
\begin{overpic}[width=\panelWidth]{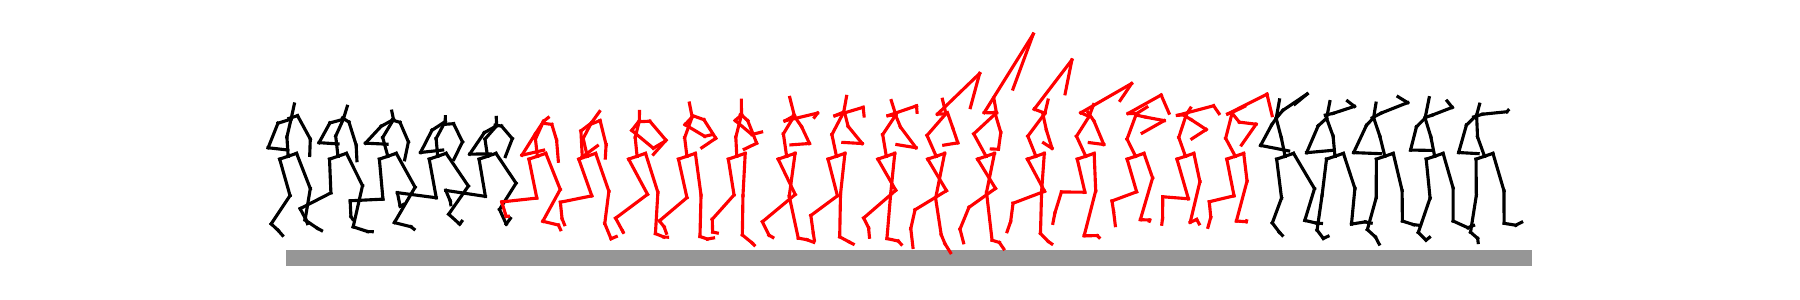}
\end{overpic} &
\begin{overpic}[width=\panelWidth]{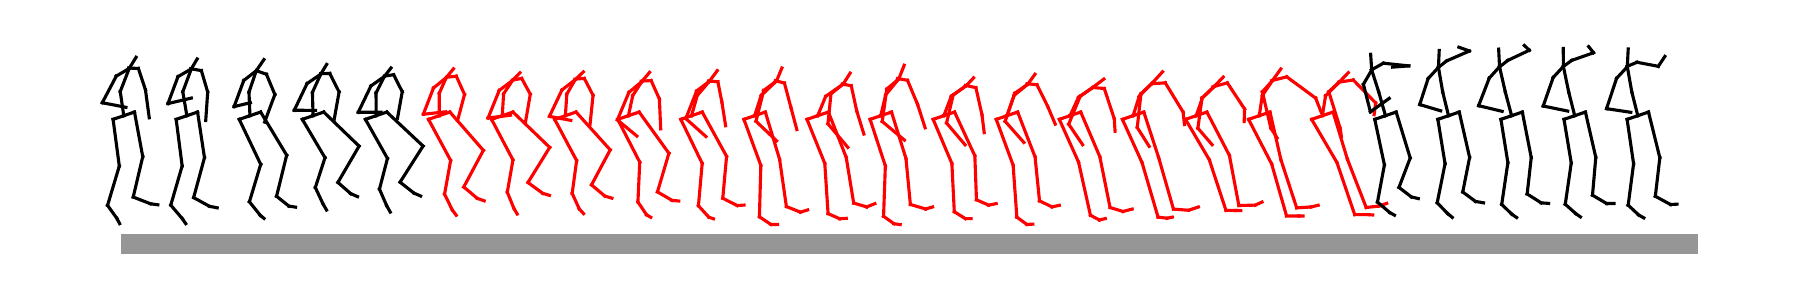}
\end{overpic}\\
\begin{overpic}[width=\panelWidth]{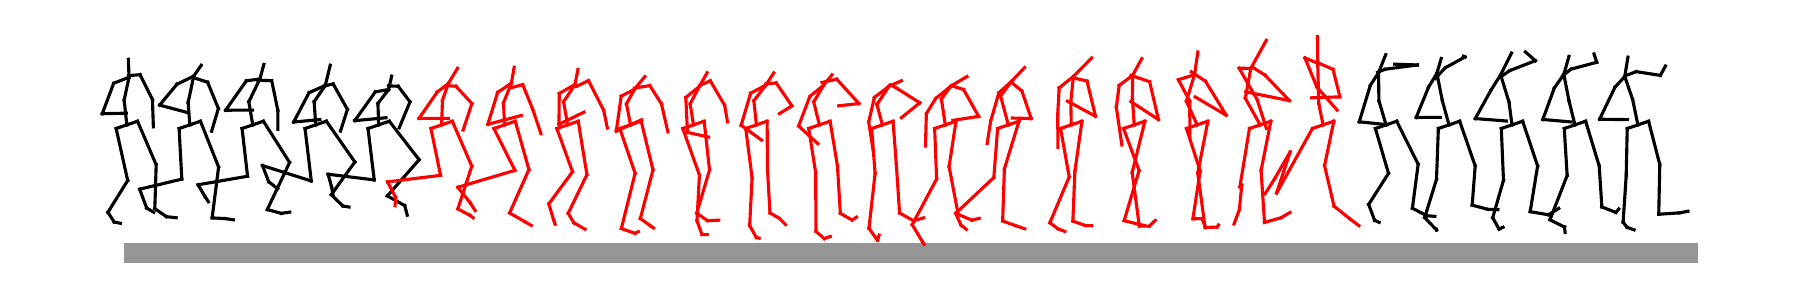}
\end{overpic} &
\begin{overpic}[width=\panelWidth]{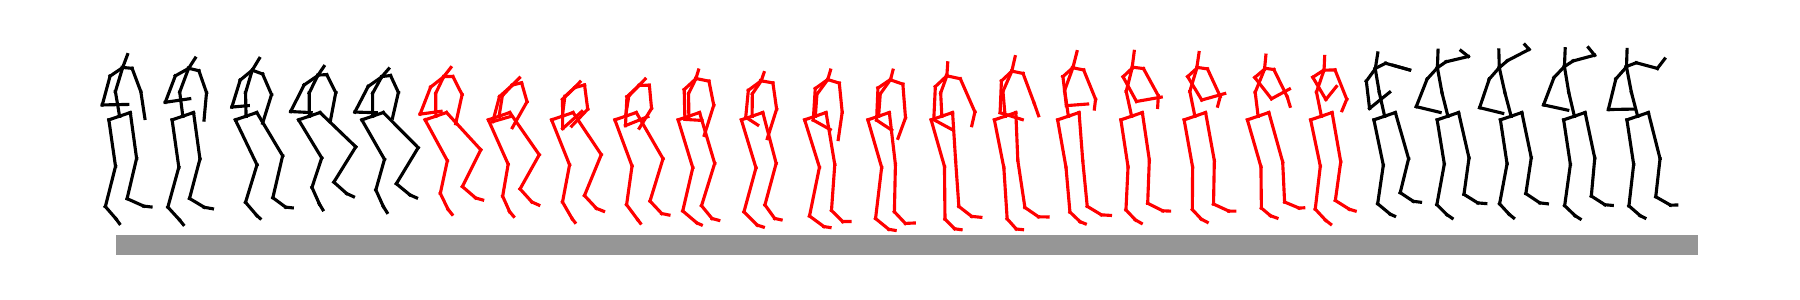}
\end{overpic} \\
\begin{overpic}[width=\panelWidth]{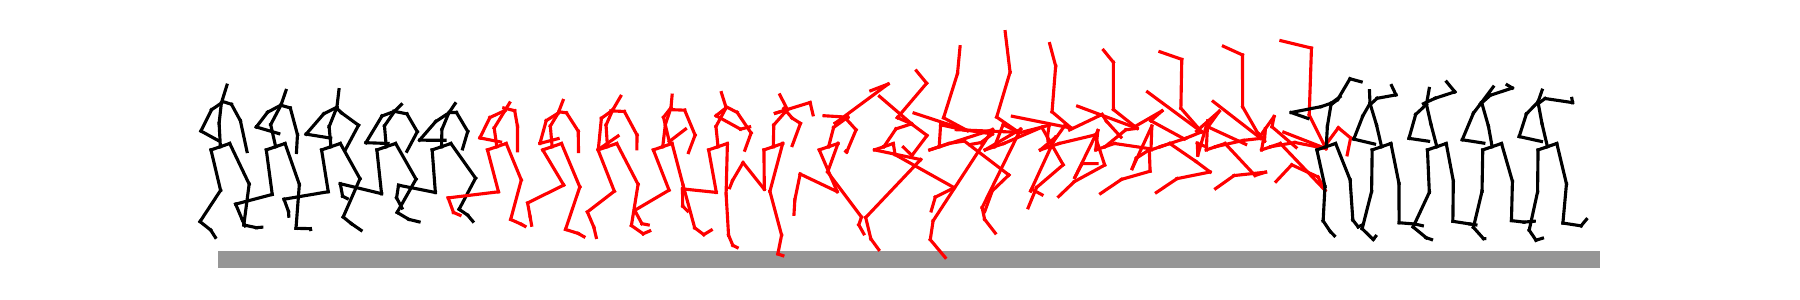}
\end{overpic} &
\begin{overpic}[width=\panelWidth]{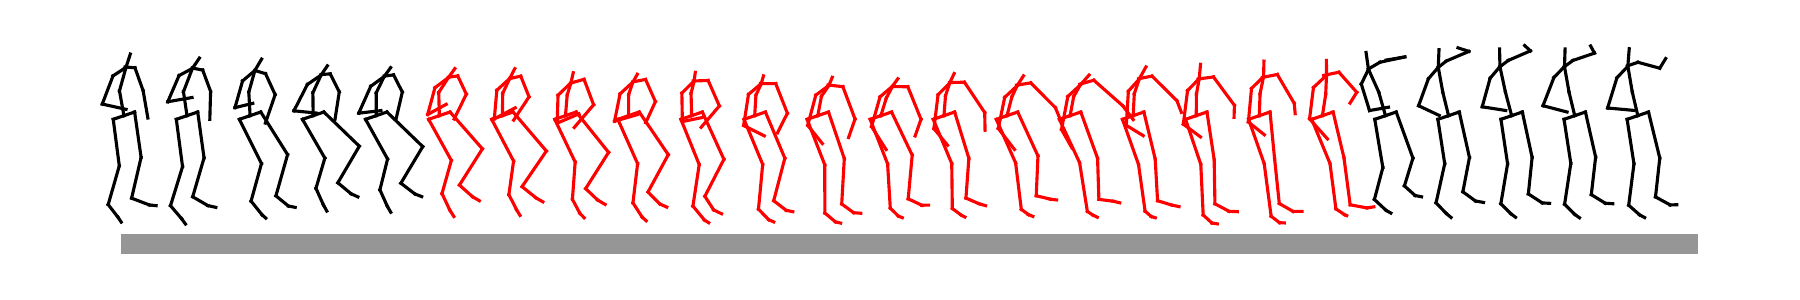}
\end{overpic}
\\
\begin{overpic}[width=\panelWidth]{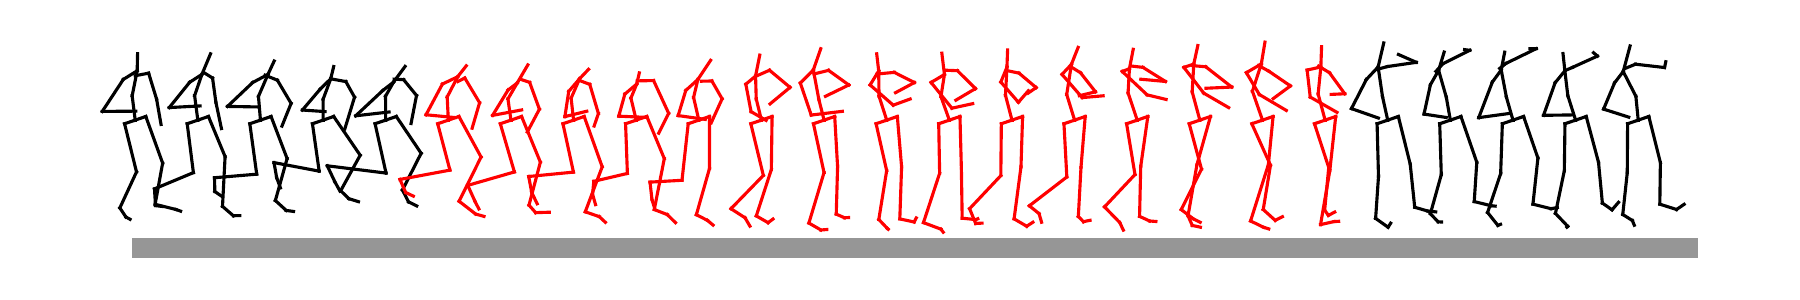}
\end{overpic} &
\begin{overpic}[width=\panelWidth]{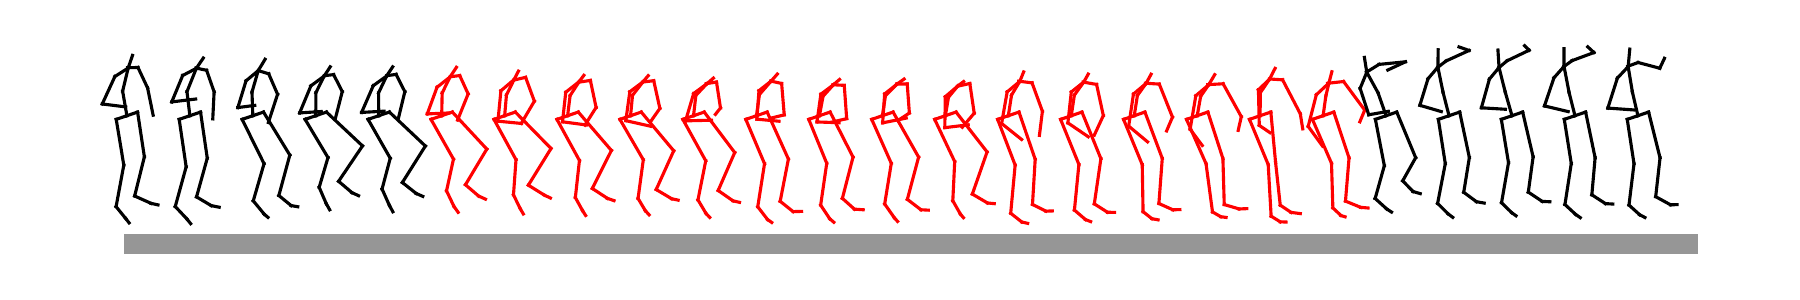}
\end{overpic}
\end{tabular}\\
(DKS+Concrete) \hspace{16mm} (DKS+Straight Through)\\
\caption[]{\small Interpolations of human motion capture data. Red figures (covering 150 time steps) are generated by each model to interpolate between the black figures four times. We see that our SVAE-SLDS provides varied plausible imputations with corresponding segmentations (colors shared with Fig.~\ref{fig:discrete}). The biased SVAE-SLDS~\cite{svae} only uses a single state and thus cannot produce diverse imputations. The autoregressive SRNN~\cite{srnn} produces varied sequences, but its inability to account for future observations prevents it from smoothly interpolating into the observed sequence end.
}
\label{fig:missing.extended}
\end{figure*}

\input{tex/F_experiment.tex}

\section{Notation}
\input{tex/E_notation.tex}

\section{Exponential families and mean field objective}
\input{tex/A_mf.tex}

\section{Belief propagation in time series}
\input{tex/B_inference.tex}

\section{Evaluating the SVAE loss}
\input{tex/C_evaluating.tex}

\section{Natural gradients}
\input{tex/D_nat.tex}

\section{Matrix-normal exponential family distributions}
\input{tex/G_ef_cat.tex}

\bibliography{svae}

\end{document}
